# Supplementary material for: Learning Transformation Synchronization
Source: arXiv:1901.09458 source file (2019-06-04)
Supplement: Supplementary file 1 [file 07_appendix.tex]

\section{Proof of Proposition 1} \label{Appendix:A}

% Algorithm \ref{Alg:laplacianRS} constructs a block matrix $L \in \mathbb{R}^{3n \times 3n}$
% % = \Bigg(
% % \begin{array}{ccccccc}
% %     d_1 I &  & \ldots & & && \\
% %      & \ddots & & & && \\
% %     \vdots & & d_i I & \ldots & -R_{ij}^T &&\\
% %     & & \vdots & \ddots & \vdots &&\\
% %     & & -R_{ij} & \ldots & d_j I &&\\
% %     & & &  & &\ddots &  \\
% %     & & & & &&d_n I
% % \end{array} \Bigg)$, i.e. a block matrix 
% with $n \times n$ blocks, the block on $i-$th row and $j-$th column is defined as 
% \begin{equation}
%     L_{ij} = \begin{cases}
%         -R_{ij} & \textup{if }(i,j) \in E\\
%         d_i I & \textup{if } i = j \\
%         0 & \textup{otherwise}
%     \end{cases}
% \end{equation}
Recall step 2 in algorithm \ref{Alg:truncated:laplacianRS} where a block matrix $A$ is constructed. In this section, we consider the noise free setting, i.e. there exists $R_1^{\star}, R_2^{\star}, \ldots R_n^{\star} \in SO(3)$, such that $R_{ij} = (R_j^{\star})^T R_i^{\star}$. We denote the block matrix constructed from perfect correspondence $R_{ij}$ as $A^{\star}$. We can write $A^{\star}$ as
\begin{equation}
    \begin{split}
        A^{\star} & \coloneqq M^T D^{-\frac{1}{2}}\tilde{A} D^{-\frac{1}{2}} M\\
        M & \coloneqq \diag(R_1^{\star}, R_2^{\star}, \ldots,  R_n^{\star}), \quad R_i^{\star} \in SO(3) \\
        D & \coloneqq \diag(d_1I, d_2I, \ldots, d_nI) \\
        \tilde{A}_{ij} & \coloneqq \begin{cases}
            I & \textup{if }(i,j) \in \set{E}\\
            0 & \textup{otherwise}
        \end{cases}
    \end{split}
    \label{eq:A0:def}
\end{equation}
The following lemma describes $A^{\star}$'s top eigenspace.
\begin{lem}
Consider $A^{\star}$ defined in \eqref{eq:A0:def}, the following holds: 
\begin{itemize}
    \item [1)] $A^{\star}$'s eigenvalues lie in $[-1, 1]$.
    \item [2)] $A^{\star}$'s eigenspace of eigenvalue 1 is 3 dimensional and can be spanned by the columns of 
    $$
        M^T D^{\frac{1}{2}} \begin{pmatrix}
        I \\
        I \\
        \vdots \\
        I
    \end{pmatrix}
    $$
\end{itemize}

\begin{proof}
1) The statement is true since $D^{-\frac{1}{2}}\tilde{A}D^{-\frac{1}{2}}$ is a normalized adjacency matrix and $M$ is orthogonal. 

2) Since $D^{-\frac{1}{2}}\tilde{A}D^{-\frac{1}{2}}$ is a normalized adjacency matrix with 3 connected components, one can show that its eigenspace of the largest eigenvalue (i.e. 1) is exactly 3 dimensional. Since 
$$
A^{\star} M^T D^{\frac{1}{2}} \begin{pmatrix}
    I \\
    I \\
    \vdots \\
    I
\end{pmatrix} = M^T D^{\frac{1}{2}}  \begin{pmatrix}
    I \\
    I \\
    \vdots \\
    I
\end{pmatrix}
$$, we confirm that the eigenspace of eigenvalue 1 can be spanned by the columns of 
$M^T D^{\frac{1}{2}} \begin{pmatrix}
    I \\
    I \\
    \vdots \\
    I
\end{pmatrix}$.
\end{proof}
\label{lem:eigenspace}
\end{lem}

Based on Lemma \ref{lem:eigenspace}, we have 
$$
B^0 \coloneqq \frac{1}{\sqrt{\sum_i d_i}} M^T D^{\frac{1}{2}} \begin{pmatrix}
    I \\
    I \\
    \vdots \\
    I
\end{pmatrix} Q = \frac{1}{\sqrt{\sum_i d_i}} \begin{pmatrix}
    \sqrt{d_1}(R_1^{\star})^T \\
    \sqrt{d_2}(R_2^{\star})^T \\
    \vdots \\
    \sqrt{d_n}(R_n^{\star})^T
\end{pmatrix} Q
$$, where $Q$ is an orthogonal matrix and the coefficient $\frac{1}{\sqrt{\sum_i d_i}}$ comes from normalization.
The algorithm then projects $\frac{\sqrt{\sum_i d_i}}{\sqrt{d_i}}(B_i^0)^T$ onto $SO(3)$, resulting in $R_i = Q^T\det(Q) R_i^{\star}$, which completes the proof of the proposition.
\section{Proof of Proposition 2}
% \input{appendix_algorithm.tex}
% \section{Proof of Theorem \ref{}}
\section{Eigenvector Stability}
\subsection{Notation and Roadmap of this section}\label{subSec:Notation}
In this section we consider a normalized adjacency matrix 
\begin{equation}
    \begin{split}
        A^{\star} &= D^{-\frac{1}{2}} \bar{A} D^{-\frac{1}{2}} \\
        D &= \diag(d_1, d_2, \ldots, d_n)
    \end{split}
\end{equation}
which is well known to have top eigenvalue $1$.
Assume the eigen-decomposition of $A^{\star}$
\begin{equation}\label{eq:Astar:eigendecomposition}
\begin{split}
    A^{\star} &= (\vec{s} | U) \Big( \begin{array}{cc}
        1 & \\
         & \Lambda
    \end{array} \Big) (\vec{s} | U)^T \\
    &= \vec{s} \vec{s}^T + U \Lambda U^T
\end{split}
\end{equation}
where $\vec{s} = \frac{1}{\sqrt{\sum_i d_i}} D^{\frac{1}{2}} \vec{1}$ is the top-eigenvector and $U$ encodes the other eigenvectors in its columns.

Consider matrix $A$ constructed in algorithm \ref{Alg:truncated:laplacianRS}, we can explicitly write it as
\begin{equation}\label{eq:A:def}
    \begin{split}
        A &= M^T A_0 M \\
        A_0 &= (A^{\star} \otimes I_3) + E \\
        E &= (D^{-\frac{1}{2}} \otimes I_3) N (D^{-\frac{1}{2}} \otimes I_3) \\
        M &= \diag(R_1^{\star}, R_2^{\star}, \ldots, R_n^{\star})
    \end{split}
\end{equation}

Note that $A$'s eigenvector stability is similar to $A_0$, therefore we consider $A_0$ first and then extend the result to $A$.

Assume $V$'s columns encode $A_0$'s top-3 eigenvectors, and let
$\Sigma = \diag(\mu_1, \mu_2, \mu_3)$ collects the top-3 eigenvalues of $A_0$. By construction, we have
\begin{equation}\label{eq:A:eigendecomposition}
    A_0 V = V \Sigma
\end{equation}
To bound the distance between $\sqrt{\sum_k d_k} (D^{-\frac{1}{2}} \otimes I_3) V$ and $\sqrt{\sum_k d_k} (D^{-\frac{1}{2}} \otimes I_3) (\vec{s} \otimes I_3)$, we write
\begin{equation}\label{eq:V:decompostion}
    V = (\vec{s} \otimes I_3) X + (U \otimes I_3) Y
\end{equation}
and for convenience also denote
\begin{equation}\label{eq:E11:E21}
    \begin{split}
        E_{11} &= (\vec{s} \otimes I_3)^T E (\vec{s} \otimes I_3) \\
        E_{21} &= (U \otimes I_3)^T E (\vec{s} \otimes I_3) \\
        E_{22} &= (U \otimes I_3)^T E (U \otimes I_3)
    \end{split}
\end{equation}

Denote $\lambda_i$ as the $i$-th largest eigenvalue of $A^{\star}$, this means if $E = 0$, $A_0$ will have eigenvalues $\{\lambda_i\}$, each with multiplicity three.

The rest of this section is organized as follows: lemma \ref{Lemma:eigenvalue:stability} introduces results for eigenvalue stability, lemma \ref{Lemma:X} controls the distance from $X$ to $O(3)$, lemma \ref{Lemma:Expression:Y} and lemma \ref{Lemma:Bound:Y} build an upper bound of $Y$, then theorem \ref{Theorem:eigenvector:stability} follows from these results.

\subsection{Main Results}
We first introduce the main result
\begin{theorem}\label{Theorem:eigenvector:stability}
    Adopting notations from Appendix \ref{subSec:Notation}, if
$$
\|E\| + \|E_{11}\| \leq \lambda_1 - \lambda_{2}
$$
    then there exists $Q \in O(3)$ so that
    \begin{equation}
        \|\sqrt{\sum_k d_k}(D^{-\frac{1}{2}} \otimes I_3)\Bigg(V - (\vec{s} \otimes I_3)Q\Bigg)\|_{2, \infty} = O(\epsilon_1 + \frac{c \epsilon_2 (1+\epsilon_1)}{1-c \epsilon_2} )
    \end{equation}
    where 
    \begin{equation} \label{eq:Notation}
    \begin{split}
        \epsilon_1 &\coloneqq  \left(\frac{\|E\|}{\lambda_1 - \lambda_{2} - \|E_{11}\|}\right)^2 \\
        \epsilon_2 &\coloneqq  \max_i \frac{1}{d_i} \sum_{(i, j) \in \set{E}} \|N_{ij}\| \\
        c &\coloneqq  \max_{\set{E_{good}} \subseteq \set{E} \subseteq \set{E_{all}}} c(\set{E}) \\
        c(\set{E}) &\coloneqq \|P_{\epsilon}\|_{1, \infty} \\
        P_{\epsilon} &\coloneqq  (D^{-\frac{1}{2}} U [(1+\epsilon)I - \Lambda] U^T D^{\frac{1}{2}}) \otimes I_3
    \end{split}
    \end{equation}
\end{theorem}

The following lemma introduced in \cite{} considers eigenvalue stability of $A_0$.
\begin{lem}\label{Lemma:eigenvalue:stability}
\textbf{(Eigenvalue Stability) \cite{}} Adopting notations from Appendix \ref{subSec:Notation}, if
$$
\|E\| + \|E_{11}\| \leq \lambda_1 - \lambda_{2}
$$, then for $1 \leq i \leq 3$, we have
\begin{equation}
    -\| E_{11} \| \leq \mu_i - \lambda_1 \leq \|E_{11} \| 
    + \frac{\| E \|^2 - \|E_{11} \|^2}{\lambda_1 - \lambda_{2}} 
\end{equation}
\end{lem}
The next lemma controls the distance from $X$ to $O(3)$.

\begin{lem}\label{Lemma:X}
\textbf{(Controlling $X$.)} Adopting notations from Appendix \ref{subSec:Notation}, 
if
$$
\|E\| + \|E_{11}\| \leq \lambda_1 - \lambda_{2}.
$$
then there exists $Q \in O(3)$ such that 
$$
    \|X - Q\| \leq 1 - \sqrt{1 - \left(\frac{\|E\|}{\lambda_1 - \lambda_{2} - \|E_{11}\|}\right)^2}
$$
in particular, 
$$
    \|X - Q\| \leq \left(\frac{\|E\|}{\lambda_1 - \lambda_{2} - \|E_{11}\|}\right)^2
$$
\end{lem}

\begin{lem}\label{Lemma:Expression:Y}
(\textbf{Expressing $Y$.}) Adopting notations from Appendix \ref{subSec:Notation} and \eqref{eq:Notation}, 
if
$$
\|E\| + \|E_{11}\| \leq \lambda_1 - \lambda_{2}
$$
Then for $1 \leq j \leq 3$, 
\begin{equation}
\begin{split}
    (U \otimes I_3) Y \vec{e}_j &= 
        \diag(\bs{s})\sum_{i=0}^{+\infty} \big(P_{\mu_j-1} D^{-1} N\big)^{i+1} (\vec{1} \otimes I_3) X \vec{e}_j
\end{split}
\label{Eq:Lambda:Expression}
\end{equation}
\end{lem}

\begin{lem}\label{Lemma:Bound:Y}
Adopting notations from Appendix \ref{subSec:Notation} and \eqref{eq:Notation}, if
$$
\|E\| + \|E_{11}\| \leq \lambda_1 - \lambda_{2}
$$
then 
\begin{equation}
\|\sqrt{\sum_k d_k}((D^{-\frac{1}{2}}U) \otimes I_3)Y\|_{2,\infty} = O(\frac{c \epsilon_2 (1 + \epsilon_1)}{1 - c \epsilon_2})
\label{Eq:Y:L:infty}
\end{equation}
\end{lem}

These four lemma is enough to prove Theorem \ref{Theorem:eigenvector:stability}.

The next lemma is to understand the term $\epsilon_1 + \frac{(1 + \epsilon_1) c \epsilon_2}{1 - c \epsilon_2}$.
\begin{lem}\label{lem:orders}
    Adopting notations from Appendix \ref{subSec:Notation} and \eqref{eq:Notation}, 
    assuming there exist constants $\rho > 0, c_2 > 0$, s.t. for all edge set $\set{E}$ with $\set{E}_{good} \subseteq \set{E} \subseteq \set{E}_{all}$
    $$
    1 - \lambda_2 - \epsilon_2 \geq \rho, \quad 1 - c \epsilon_2 \geq c_2
    $$
    we have
    \begin{align*}
        \epsilon_2 \leq 2, \quad \epsilon_1 \leq \frac{\epsilon_2^2}{\rho^2}
    \end{align*}
    and
    \begin{align*}
        \epsilon_1 + \frac{(1 + \epsilon_1) c \epsilon_2}{1 - c \epsilon_2} &\leq \frac{\epsilon_2^2}{\rho^2} + \frac{(1+\frac{\epsilon_2^2}{\rho^2}) c \epsilon_2}{c_2} \\
        &\leq (\frac{2}{\rho^2} + \frac{c(1+\frac{4}{\rho^2})}{c_2}) \epsilon_2
    \end{align*}
\end{lem}
The proof of this lemma is omitted.

We then begins to bound $\|R_i^t - Q^TR_i^{\star}\|$ for each iteration $t$ in the algorithm.
\begin{lem}\label{Lemma:delta} Adopting notations from Appendix \ref{subSec:Notation} and \eqref{eq:Notation}. Consider algorithm \ref{Alg:truncated:laplacianRS}, we first define
\begin{itemize}
    \item Let $\set{E}^{(t)}$ be the edge set before the $t$-th iteration, e.g. $\set{E}^{(0)} = \set{E}_{all}$, and $R_i^{(t)}$ be the value of $R_i$ after $t$-th iteration.
    \item Let 
    $$
    \epsilon_2^{(t)} \coloneqq \max_i \frac{1}{d_i} \sum_{(i, j) \in \set{E}^{(t)}} \|N_{ij}\|
    $$
    ,
    $$
        \delta^{(t)} \coloneqq \min_{Q \in O(3)}\max_i \|R_i^{(t)} - Q^T R_i^{\star}\|
    $$
    ,
    $$
        C^{(t)} \coloneqq \max_{(i, j) \in \set{E}^{(t)}} \|N_{ij}\|
    $$
    ,
    $$
        c_3 \coloneqq (\frac{2}{\rho^2} + \frac{3 c(1+\frac{4}{\rho^2})}{c_2}) + 2 (\frac{2}{\rho^2} + \frac{3 c(1+\frac{4}{\rho^2})}{c_2})^2
    $$,
    $$
        r \coloneqq \frac{d_{bad}}{d_{good}}
    $$
\end{itemize}, then the following holds
\begin{itemize}
    \item For the first iteration,
    \begin{align}
        C^{(0)} &\leq C \\
        \epsilon_2^{(0)} &\leq \sigma + C \\
        \delta^{(0)} &\leq c_3(\sigma + C) \\
        C^{(1)} &\leq \epsilon_0 + c_3 \sigma + r c_3 C
    \end{align}
    \item For $t \geq 1$, if 
    $$
    C^{(t)} \leq (\sum_{i=0}^{t-1} (rc_3)^i \tilde{c}^{t-i-1}) \epsilon_0 + c_3(\frac{1-(rc_3)^t}{1-rc_3}) \sigma + (rc_3)^t C
    $$, then
    \begin{align}
        \epsilon_2^{(t)} &\leq \sigma + r C^{(t)} \\
        & = r(\sum_{i=0}^{t-1} (rc_3)^i \tilde{c}^{t-i-1}) \epsilon_0  \\
        &+ (r c_3(\frac{1-(rc_3)^t}{1-rc_3}) + 1) \sigma + r (rc_3)^t C \\
        \delta^{(t)} &\leq c_3 \epsilon_2^{(t)} \\
        C^{(t+1)} &\leq \epsilon_0 \tilde{c}^{t-1} + \delta^{(t)} \\
        & \leq \epsilon_0 \tilde{c}^{t-1} + c_3 \epsilon_2^{(t)} \\
        &\leq [(\sum_{i=0}^{t-1} (rc_3)^{i+1} \tilde{c}^{t-i-1}) + \tilde{c}^{t-1}] \epsilon_0  \\
        &+ c_3(r c_3(\frac{1-(rc_3)^t}{1-rc_3}) + 1) \sigma + (rc_3)^{t+1} C \\
        &\leq [(\sum_{i=1}^{t} (rc_3)^{i} \tilde{c}^{t-i}) + \tilde{c}^{t-1}] \epsilon_0  \\
        &+ c_3\frac{1-(rc_3)^{t+1}}{1-rc_3} \sigma + (rc_3)^{t+1} C \\
        &\leq (\sum_{i=0}^{t} (rc_3)^{i} \tilde{c}^{t-i}) \epsilon_0  \\
        &+ c_3\frac{1-(rc_3)^{t+1}}{1-rc_3} \sigma + (rc_3)^{t+1} C
    \end{align}    
\end{itemize}
    % Let the maximum degree be $d_{\max}$, the minimal number of correct edges for each node be $d_{\textup{good}}$.
    % Define $\delta(\set{E})$ w.r.t. the current edge set $\set{E}$ as
    % $$
    %     \delta(\set{E}) \coloneqq \min_{Q \in O(3)} \max_{i} \|R_i - Q^T R_i^{\star}\|
    % $$
    % we have
    % \begin{equation}
    %     \delta(\set{E}) = O(\epsilon_1 + \frac{c \epsilon_2}{1-c \epsilon_2} (1+\epsilon_1))
    % \end{equation}

\end{lem}

\subsection{Proof of Key Lemmas}
\subsubsection{Proof of Lemma \ref{Lemma:Expression:Y}}

\begin{proof}
    From \eqref{eq:A:eigendecomposition} we have
    $$
        A_0 V = V \Sigma,
    $$
    apply \eqref{eq:V:decompostion}, we have
    $$
        A_0 ((\vec{s} \otimes I_3) X + (U \otimes I_3) Y) = ((\vec{s} \otimes I_3) X + (U \otimes I_3) Y) \Sigma
    $$
    multiply $(U \otimes I_3)^T$ from the left and apply \eqref{eq:A:def}, we have
    \begin{align}
        (U \otimes I_3)^T (A^{\star} \otimes I_3 + E) ( (\vec{s} \otimes I_3) X + (U \otimes I_3) Y) = Y \Sigma
    \end{align}
    applying \eqref{eq:E11:E21} leads to
    \begin{align}
        (\Lambda \otimes I_3) Y + E_{21} X + E_{22} Y  = Y \Sigma
    \end{align}
    for $j = 1, \ldots, 3$, multiply $\vec{e}_j$ from the right, we have
    \begin{align}
        ((\mu_j I - \Lambda \otimes I_3) - E_{22})) Y \vec{e}_j = E_{21} X \vec{e}_j
    \end{align} 
    from Lemma \ref{Lemma:eigenvalue:stability}, we have
    \begin{align}
        \|E_{22}\| &\leq \|E\| \\
        & \leq \lambda_1 - \lambda_2 - \|E_{11}\| \\
        & \leq \mu_j - \lambda_2 \\
        & \leq \|\mu_j I - (\Lambda \otimes I_3)\|
    \end{align}
    which guarantees the validity of the following Taylor expansion
    \begin{align}
        Y \vec{e}_j &= ((\mu_j I - \Lambda \otimes I_3) - E_{22}))^{-1}E_{21} X \vec{e}_j \\
        &= ((\mu_j I - \Lambda \otimes I_3)(I - (\mu_j I - \Lambda \otimes I_3)^{-1} E_{22}))^{-1} E_{21} X \vec{e}_j \\
        &= (I - (\mu_j I - \Lambda \otimes I_3)^{-1} E_{22})^{-1} (\mu_j I - \Lambda \otimes I_3)^{-1} E_{21} X \vec{e}_j \\
        &= \sum_{i=0}^{+\infty} ((\mu_j I - \Lambda \otimes I_3)^{-1} E_{22})^i (\mu_j I - \Lambda \otimes I_3)^{-1} E_{21} X \vec{e}_j
    \end{align}
    Multiply $(U \otimes I_3)$ from the left on both side and let $P_{\epsilon} =  (D^{-\frac{1}{2}} U [(1+\epsilon)I - \Lambda] U^T D^{\frac{1}{2}}) \otimes I_3$, we have
    \begin{align}
        &~~~~~(U \otimes I_3) Y \vec{e}_j \nonumber \\
        &= \sum_{i=0}^{+\infty} D^{\frac{1}{2}} (P_{\mu_j-1} D^{-1} N)^{i+1} D^{-\frac{1}{2}} (\vec{s} \otimes I_3) X \vec{e}_j \nonumber \\
        &= \frac{1}{\sqrt{\sum_k d_k}} \sum_{i=0}^{+\infty} D^{\frac{1}{2}} (P_{\mu_j-1} D^{-1} N)^{i+1} (\vec{1} \otimes I_3) X \vec{e}_j\nonumber \\
        &= \diag(\bs{s})\sum_{i=0}^{+\infty} \big(P_{\mu_j-1} D^{-1} N\big)^{i+1} (\vec{1} \otimes I_3) X \vec{e}_j
    \end{align}
\end{proof}

\subsubsection{Proof of Lemma \ref{Lemma:Bound:Y}}
\begin{proof}
From Lemma \ref{Lemma:Expression:Y}, 
    \begin{align*}
        &~~\|\sqrt{\sum_k d_k} ((D^{-\frac{1}{2}}U) \otimes I_3) Y \vec{e}_j \|_{\infty} \\
        &\leq \sum_{i=0}^{+\infty} \|\diag(\bs{1}) \big(P_{\mu_j-1} D^{-1} N\big)^{i+1} (\vec{1} \otimes I_3) X \vec{e}_j\|_{\infty} \\
        &\leq \sum_{i=0}^{+\infty} \|\diag(\bs{1})\|_{1, \infty} \|\big(P_{\mu_j-1} D^{-1} N\big)^{i+1}\|_{1, \infty} \|X\| \\
        &\leq \sum_{i=0}^{+\infty}  \|\big(P_{\mu_j-1} D^{-1} N\big)\|_{1, \infty}^{i+1} \|X\| \\
        &= \frac{\|P_{\mu_j-1} D^{-1} N\|_{1, \infty} \|X\| }{1-\|P_{\mu_j-1} D^{-1} N\|_{1, \infty}}\\
        &\leq \frac{\|P_{\mu_j-1} \|_{1, \infty} \|D^{-1} N \|_{1, \infty} \|X\| }{1-\|P_{\mu_j-1} \|_{1, \infty} \|D^{-1} N\|_{1, \infty}} \\
        &\leq \frac{\|P_{\mu_j-1} \|_{1, \infty} \max_i \frac{\sqrt{3}}{d_i} \sum_{j \in \partial{i}} \|N_{ij}\| \|X\| }{1-\|P_{\mu_j-1} \|_{1, \infty} \max_i \frac{\sqrt{3}}{d_i} \sum_{j \in \partial{i}} \|N_{ij}\|} 
    \end{align*}
Let 
\begin{align*}
    c(\set{E}) &\coloneqq \sqrt{3} \max_{\epsilon \in \set{D}}\|P_{\epsilon}\|_{1, \infty} \\
    \set{D} &\coloneqq \big[-\|E_{11}\|,~  \|E_{11}\| + \frac{\|E\|^2 - \|E_{11}\|^2}{1 - \lambda_2}\big] \\
    c &\coloneqq \max_{\set{E}_{good} \subseteq \set{E} \subseteq \set{E}_{all}}c(\set{E}) \\
    \epsilon_2 &\coloneqq \max_i \frac{1}{d_i} \sum_{j \in \partial{i}} \|N_{ij}\|
\end{align*}
and recall lemma \ref{Lemma:X}, we get
    \begin{align*}
        \|\sqrt{\sum_k d_k} ((D^{-\frac{1}{2}}U) \otimes I_3) Y \vec{e}_j \|_{\infty} &\leq \frac{c \epsilon_2 (1+\epsilon_1) }{1- c \epsilon_2 }
    \end{align*}
Combine the results for $1 \leq j \leq 3$, we have
\begin{align*}
    \|\sqrt{\sum_k d_k} ((D^{-\frac{1}{2}}U) \otimes I_3) Y \|_{2, \infty} &\leq \frac{\sqrt{3} c \epsilon_2 (1+\epsilon_1) }{1-c \epsilon_2 }
\end{align*}
\end{proof}

\subsubsection{Proof of Theorem \ref{Theorem:eigenvector:stability}}
\begin{proof}

Note that
\begin{align*}
    \|X - Q\| &\leq \frac{\|E\|^2}{(1 - \lambda_2 - \|E_{11}\|)^2} \nonumber \\
    & \leq \frac{\|D^{\frac{1}{2}}\|^2 \|(D^{-1}\otimes I_3) N\|^2 \|D^{-\frac{1}{2}}\|^2}{(1 - \lambda_2 - \|E_{11}\|)^2} \nonumber \\
    & \leq \frac{d_{\max} \epsilon_2^2}{d_{\min}(1 - \lambda_2 - \epsilon_2)^2} \nonumber \\
    & \leq \frac{d_{\max} \epsilon_2^2}{d_{\min}(\rho - \epsilon_2)^2}
\end{align*}
where 
$$
    \rho \coloneqq \min_{\set{E}_{good} \subseteq \set{E} \subseteq \set{E}_{all}} 1 - \lambda_2(\set{E})
$$
From \eqref{eq:V:decompostion} and lemma \ref{Lemma:X}, we have
\begin{align*}
    &~~~~~\|\sqrt{\sum_k d_k} (D^{-\frac{1}{2}} \otimes I_3) \Big[ V - (\vec{s} \otimes I_3)Q \Big] \|_{2, \infty}  \\
    &= \|(\vec{1} \otimes I_3)(X-Q) + \sqrt{\sum_k d_k} ((D^{-\frac{1}{2}}U) \otimes I_3)Y\|_{2, \infty} 
    \\
    & \leq \|(\vec{1} \otimes I_3)\|_{2, \infty} \|(X-Q)\| + \frac{c \epsilon_2 (1+\epsilon_1) }{1-c \epsilon_2 } \\
    & \leq  \epsilon_1 + \frac{\sqrt{3} c \epsilon_2 (1+\epsilon_1) }{1-c \epsilon_2 }
\end{align*}
\end{proof}
\section{Derivatives of SVD}

\noindent \textbf{Proof of Proposition \ref{Prop:Rot:Sync:Recovery}.}

Suppose the constraints (\ref{Eq:Rotation:Recovery:Condition} are exact. We construct a matrix $B\in\mathbb{R}^{3|\set{E}|\times 3n}$. $B$ is consisting of $|\set{E}|\times n$ submatrices $B_{ij}$ each having size $3\times 3$. Each edge $e_k$ in $\set{E}$ corresponds to 3 rows in $B$, or a row of $B_{kl}$, and each vertex in $\set{G}$ corresponds to a column in $B$. If $e_k=(i,j)\in\set{E}$, then there will be two non-zero items in $B_{kl}$ such that
$$
B_{k i}=\sqrt{w_{ij}}{R_i^{gt}}^T,\ B_{k j}=-\sqrt{w_{ij}}{R_j^{gt}}^T
$$

It is worth noting that $\set{E}$ is an undirected edge set so there can be two alternatives for an edge to fill out a row of $B_{kl}$. However we would see this uncertainty does not affect our results. If $i=j$ then
$$
[B^TB]_{ii}=\sum_{k=1}^nB_{ki}^TB_{ki}=\sum_{j\in \set{N}(i)}w_{ij}I_3.
$$
If $(i,j)\in\set{E}$ then
\begin{align*}
[B^TB]_{ij}&=\sum_{k=1}^nB_{ki}^TB_{kj}\\
&=-w_{ij}{R_i^{gt}}{R_j^{gt}}^T\\
&=-w_{ij}R_{ji}\\
&=-w_{ij}R_{ij}^T=L_{ij} .
\end{align*}
Otherwise it can be easily seen that $[B^TB]_{ij}=0$. Anyway we verified that $L=B^TB$. This factorization means $L$ is semi-definite positive.

On the other hand, if $(i,j)\in\set{E}$
$$
L_{ij}R_j=-w_{ij}R_{ij}^TR_j=-w_{ij}R_{ji}R_j=-w_{ij}R_i.
$$

Together with $L_{ij}R_i=\sum_{j\in\set{N}(i)}w_{ij}R_i$, we have
$$
L\begin{bmatrix}
R_1\\
\vdots\\
R_n
\end{bmatrix}
=0.
$$
Thus $L$ contains at least 3 zero eigenvalues. In fact it contains exactly 3 ones if $\set{G}$ is a connected graph. Suppose $L\bs{u}=0$ for some vector $\bs{u}\in\mathbb{R}^{3n}$ and $\bs{u}=[\bs{u}_1^T,\dots,\bs{u}_n^T]^T$. Substituting $L=B^TB$ into it we obtain
$$
\bs{u}^TB^TB\bs{u}=\|Bu\|^2=0.
$$
Rewriting this formula in blockwise form we have
$$
\sum_{(i,j)\in\set{E}}\|R_i^T\bs{u}_i-R_j^T\bs{u}_j\|^2=0.
$$
Hence $R_i^T\bs{u}_i=R_j^T\bs{u}_j$. Since we have assumed $\set{G}$ is connected, $R_i^T\bs{u}_i$ must be a constant for all $i=1,\dots,n$. Letting $\bs{z}=R_i^T\bs{u}_i$ immediately gives $\bs{u}_i=R_i\bs{z}$, or
$$
\bs{u}=\begin{bmatrix}
R_1\\
\vdots\\
R_n
\end{bmatrix}
\bs{z}
$$
where $\bs{z}\in\mathbb{R}^{3}$. But this implies $\bs{u}$ is just a linear combination of $\bs{z}$. Combining with the proved fact that $L$ is semi-positive definite, we conclude
$$
0=\sigma_1=\sigma_2=\sigma_3<\sigma_4<\dots
$$

\noindent\textbf{Comment.} The sub-matrix size $3\times 3$ can be generalized to general $k\times k$ matrix with the exactly same argument.

The

\begin{proposition}
Suppose $L$ is an $nk$-by-$nk$ symmetric matrix. The eigen-decomposition of $L$ is
$$
L=W\Lambda W^T
$$
where $W=[\bs{w}_1,\dots,\bs{w}_{nk}],\ \Lambda=\diag(\lambda_1,\dots,\lambda_{nk})$ and $\Lambda$ is reordered so that $$\lambda_1\leq \dots\leq\lambda_k<\lambda_{k+1}\leq \dots\leq \lambda_{nk}.$$
Note that we assumed a spectral gap between $\lambda_k$ and $\lambda_{k+1}$.
We also write $W_k=[\bs{w}_1,\dots,\bs{w}_k]$ to denote the first $k$ eigenvectors. The $k$-by-$k$ blocks along $W_k$ can be listed as following
$$
A_i=(\bs{e}_i^T\otimes I_m)W,\quad i=1,\dots,n.
$$
Do singular value decomposition (or SVD) on $A_i$ gives
$$
A_i=U^{(i)}\Sigma^{(i)}{V^{(i)}}^T
$$
and by definition \ref{def:rotation} we have
$$
R_i=R(A_i)=U^{(i)}{V^{(i)}}^T.
$$
Specifically, we write $U^{(i)},V^{(i)},\Sigma^{(i)}$ in detail,
\begin{align*}
U^{(i)}&=[\bs{u}^{(i)}_1,\dots,\bs{u}^{(i)}_k],\\
V^{(i)}&=[\bs{v}^{(i)}_1,\dots,\bs{v}^{(i)}_k],\\
\Sigma^{(i)}&=\diag(\sigma^{(i)}_1,\dots,\sigma^{(i)}_k).
\end{align*}
To avoid confusion, we use $\bs{e}_i^{(k)}$ to denote the unit $k$-length vector with the $i$th row being one and others being zero. Based on these notations, the differential follows:
\begin{equation}
    \dd (R_iR_j^T)=\dd R_i^{(outer)}R_j^T+R_i\dd {R_j^{(outer)}}^T
\end{equation}
where
\begin{align}
\dd R_i^{(outer)}&=\sum_{1\leq s,t,j\leq k}\sum_{l=k+1}^{kn}\frac{\bs{w}_j^T\dd L\bs{w}_l\bs{u}_s^{(i)}{\bs{v}_t^{(i)}}^T}{(\sigma_s^{(i)}+\sigma_t^{(i)})(\lambda_j-\lambda_l)}\times \nonumber \\
&\qquad\Big(\big((\bs{e}_i^{(n)}\otimes I_k)\bs{u}_s^{(i)}\big)^T\bs{w}_l{\bs{e}_j^{(k)}}^T\bs{v}_t^{(i)}-\nonumber\\
&\qquad\qquad\big((\bs{e}_i^{(n)}\otimes I_k)\bs{u}_t^{(i)}\big)^T\bs{w}_l{\bs{e}_j^{(k)}}^T\bs{v}_s^{(i)}\Big).
\label{eq:derivative:14}
\end{align}
Note that since $\lambda_j<\lambda_l$ for all $j\leq k<l$ hence (\ref{eq:derivative:14}) is well-defined and computable.
\end{proposition}

\begin{proof}

\end{proof}
\input{app_03_more_experiments.tex}

\section{Empirical Graph Connectivity}
In this section, we sample scenes from both Redwood and Scannet dataset and plot the error distribution on the graph of 30 scans. In the following figures, each edge represents a relative pose established from either Super4PCS or Fast Global Registration. The line width of edges reflects the errors of this relative pose. In order to successfully recover ground truth poses, recovery algorithms need to downweight edges that have large errors without hurting graph connectivity. We compare baseline algorithms and our approach on this procedure.
