# Supplementary material for: Learning Transformation Synchronization
Source: arXiv:1901.09458 source file (2019-06-04)
Supplement: Supplementary file 2 [file appendix_algorithm.tex]

\section{Truncated Rotation Synchronization Algorithm}

\begin{algorithm}[H]
    \caption{Truncated Rotation Synchronization}
    \begin{algorithmic}
        \State \textbf{Input:} Number of nodes $n$, edge set $\set{E}$, correspondences $R_{ij}, ~~ \forall (i, j) \in \set{E}$, initial error threshold $\epsilon_0 > 0$, decay factor $c \in (0, 1)$.
        \State \textbf{Parameter:} Initial threshold $c$, threshold step size $\alpha$.
        \State 1. Initialize weights $\vec{w}^0 \in \R^{|\set{E}|}$, where each edge $(i,j)\in\set{E}$ has an associated weight $w_{ij}$. Assign $$w_{ij}^0 \gets 1, \quad \forall (i, j) \in \set{E}$$
        \For{$t = 0, 1, \ldots $}
        \State 2. Compute (weighted) degree of each node $i$.
        $$d_i^t \gets \sum_j w_{ij}^t$$
        \State 3. Construct sparse block matrix
        \begin{equation}
            \begin{split}
                A & = 
                \begin{pmatrix}
                    A_{11} & A_{12} & \ldots & A_{1n} \\
                    A_{21} & A_{22}& \ldots & A_{2n} \\
                    \vdots & & \ddots & \vdots\\
                    A_{n1} & A_{n2} & \ldots & A_{nn}
                \end{pmatrix}
                , \\
                s.t.~~ A_{ij} &= 
                \begin{cases}
                    \frac{w_{ij}^t}{\sqrt{d_i d_j}}R_{ij}^T & \textup{if }(i, j) \in \set{E} \\ 
                    0 & \textup{otherwise}
                \end{cases}
            \end{split}
            \label{eq:A:construct}
        \end{equation}
        \State 4. Compute top three eigenvectors of $A$, denoted as columns of $B = \begin{pmatrix}
            B_1 \\
            B_2 \\
            \vdots \\
            B_n
        \end{pmatrix} \in \mathbb{R}^{3n \times 3}$ where $B_i \in \mathbb{R}^{3 \times 3}$ and let 
        $$
        V = \sqrt{\sum_k d_k} (D^{-\frac{1}{2}} \otimes I_3) \begin{pmatrix}
            B_1^T \\
            B_2^T \\
            \vdots \\
            B_n^T
        \end{pmatrix} =  
        \begin{pmatrix}
            \frac{\sqrt{\sum_i d_i}}{\sqrt{d_1}}B_1^T \\
            \frac{\sqrt{\sum_i d_i}}{\sqrt{d_2}}B_2^T \\
            \vdots \\
            \frac{\sqrt{\sum_i d_i}}{\sqrt{d_n}}B_n^T
        \end{pmatrix}
        $$
        
        \State 5. Take SVD of $V_i$ as $U_i \Sigma_i W_i^T$. Then assign
        $$
        R_i \gets \frac{1}{\det(U_i W_i^T)} U_i W_i^T
        $$.
        \State 6. Compute translations $\bs{t}_i$ by solving
            $\min_{\bs{t}_i} \sum_{i, j \in \set{E}} \| \bs{t}_i - \bs{t}_j - R_j \bs{t}_{ij}\|^2$
        \State 7. Compute $\vec{w}^{t+1}$ as follows: \\
        $$
        \forall (i, j) \in \set{E}, \quad w_{ij}^{t+1} \gets \begin{cases}
            0 & \textup{if }  \|R_j^T R_i - R_{ij}\|_{\mathcal{F}} > \epsilon_0 \alpha^t \textup{ or } \|\bs{t}_i - \bs{t}_j - R_j \bs{t}_{ij}\| > \epsilon_0 \alpha^t \\
            1 & \textup{otherwise }
        \end{cases}
        $$
        \EndFor
        
        \State \textbf{Output: $\{R_i\}$}
    \end{algorithmic}
    \label{Alg:truncated:laplacianRS}
\end{algorithm}

In practice we can expect some of the measurements over graph $\set{G}=(\set{V}(\set{G}),\set{E}(\set{G}))$ is relatively accurate with reasonable errors but others could be far away from the ground truth. In the deterministic setting We use a subgraph $\set{G}_{good}$ of $\set{G}$ to model such behavior. Particularly
\begin{equation}
    \|R_{ij}\|\leq
    \begin{cases}
    \sigma,&\ \textup{if } (i,j)\in\set{E}(\set{G}_{good})\\
    C,&\ \textup{if } (i,j)\in \set{E}(\set{G})\setminus\set{E}(\set{G}_{good})
    \end{cases}
\end{equation}
Of course the constraint $R_{ij}=R_{ji}^T$ still holds true. The following theorem states that Algorithm \ref{Alg:truncated:laplacianRS} could reach a good approximation of the ground truth rotations.

\begin{theorem}
    
\end{theorem}

\begin{proof}

\end{proof}
