# Supplementary material for: Learning Transformation Synchronization
Source: arXiv:1901.09458 source file (2019-06-04)
Supplement: Supplementary file 3 [file appendix_derivatives.tex]

\section{Derivatives of SVD}

\noindent \textbf{Proof of Proposition \ref{Prop:Rot:Sync:Recovery}.}

Suppose the constraints (\ref{Eq:Rotation:Recovery:Condition} are exact. We construct a matrix $B\in\mathbb{R}^{3|\set{E}|\times 3n}$. $B$ is consisting of $|\set{E}|\times n$ submatrices $B_{ij}$ each having size $3\times 3$. Each edge $e_k$ in $\set{E}$ corresponds to 3 rows in $B$, or a row of $B_{kl}$, and each vertex in $\set{G}$ corresponds to a column in $B$. If $e_k=(i,j)\in\set{E}$, then there will be two non-zero items in $B_{kl}$ such that
$$
B_{k i}=\sqrt{w_{ij}}{R_i^{gt}}^T,\ B_{k j}=-\sqrt{w_{ij}}{R_j^{gt}}^T
$$

It is worth noting that $\set{E}$ is an undirected edge set so there can be two alternatives for an edge to fill out a row of $B_{kl}$. However we would see this uncertainty does not affect our results. If $i=j$ then
$$
[B^TB]_{ii}=\sum_{k=1}^nB_{ki}^TB_{ki}=\sum_{j\in \set{N}(i)}w_{ij}I_3.
$$
If $(i,j)\in\set{E}$ then
\begin{align*}
[B^TB]_{ij}&=\sum_{k=1}^nB_{ki}^TB_{kj}\\
&=-w_{ij}{R_i^{gt}}{R_j^{gt}}^T\\
&=-w_{ij}R_{ji}\\
&=-w_{ij}R_{ij}^T=L_{ij} .
\end{align*}
Otherwise it can be easily seen that $[B^TB]_{ij}=0$. Anyway we verified that $L=B^TB$. This factorization means $L$ is semi-definite positive.

On the other hand, if $(i,j)\in\set{E}$
$$
L_{ij}R_j=-w_{ij}R_{ij}^TR_j=-w_{ij}R_{ji}R_j=-w_{ij}R_i.
$$

Together with $L_{ij}R_i=\sum_{j\in\set{N}(i)}w_{ij}R_i$, we have
$$
L\begin{bmatrix}
R_1\\
\vdots\\
R_n
\end{bmatrix}
=0.
$$
Thus $L$ contains at least 3 zero eigenvalues. In fact it contains exactly 3 ones if $\set{G}$ is a connected graph. Suppose $L\bs{u}=0$ for some vector $\bs{u}\in\mathbb{R}^{3n}$ and $\bs{u}=[\bs{u}_1^T,\dots,\bs{u}_n^T]^T$. Substituting $L=B^TB$ into it we obtain
$$
\bs{u}^TB^TB\bs{u}=\|Bu\|^2=0.
$$
Rewriting this formula in blockwise form we have
$$
\sum_{(i,j)\in\set{E}}\|R_i^T\bs{u}_i-R_j^T\bs{u}_j\|^2=0.
$$
Hence $R_i^T\bs{u}_i=R_j^T\bs{u}_j$. Since we have assumed $\set{G}$ is connected, $R_i^T\bs{u}_i$ must be a constant for all $i=1,\dots,n$. Letting $\bs{z}=R_i^T\bs{u}_i$ immediately gives $\bs{u}_i=R_i\bs{z}$, or
$$
\bs{u}=\begin{bmatrix}
R_1\\
\vdots\\
R_n
\end{bmatrix}
\bs{z}
$$
where $\bs{z}\in\mathbb{R}^{3}$. But this implies $\bs{u}$ is just a linear combination of $\bs{z}$. Combining with the proved fact that $L$ is semi-positive definite, we conclude
$$
0=\sigma_1=\sigma_2=\sigma_3<\sigma_4<\dots
$$

\noindent\textbf{Comment.} The sub-matrix size $3\times 3$ can be generalized to general $k\times k$ matrix with the exactly same argument.

The

\begin{proposition}
Suppose $L$ is an $nk$-by-$nk$ symmetric matrix. The eigen-decomposition of $L$ is
$$
L=W\Lambda W^T
$$
where $W=[\bs{w}_1,\dots,\bs{w}_{nk}],\ \Lambda=\diag(\lambda_1,\dots,\lambda_{nk})$ and $\Lambda$ is reordered so that $$\lambda_1\leq \dots\leq\lambda_k<\lambda_{k+1}\leq \dots\leq \lambda_{nk}.$$
Note that we assumed a spectral gap between $\lambda_k$ and $\lambda_{k+1}$.
We also write $W_k=[\bs{w}_1,\dots,\bs{w}_k]$ to denote the first $k$ eigenvectors. The $k$-by-$k$ blocks along $W_k$ can be listed as following
$$
A_i=(\bs{e}_i^T\otimes I_m)W,\quad i=1,\dots,n.
$$
Do singular value decomposition (or SVD) on $A_i$ gives
$$
A_i=U^{(i)}\Sigma^{(i)}{V^{(i)}}^T
$$
and by definition \ref{def:rotation} we have
$$
R_i=R(A_i)=U^{(i)}{V^{(i)}}^T.
$$
Specifically, we write $U^{(i)},V^{(i)},\Sigma^{(i)}$ in detail,
\begin{align*}
U^{(i)}&=[\bs{u}^{(i)}_1,\dots,\bs{u}^{(i)}_k],\\
V^{(i)}&=[\bs{v}^{(i)}_1,\dots,\bs{v}^{(i)}_k],\\
\Sigma^{(i)}&=\diag(\sigma^{(i)}_1,\dots,\sigma^{(i)}_k).
\end{align*}
To avoid confusion, we use $\bs{e}_i^{(k)}$ to denote the unit $k$-length vector with the $i$th row being one and others being zero. Based on these notations, the differential follows:
\begin{equation}
    \dd (R_iR_j^T)=\dd R_i^{(outer)}R_j^T+R_i\dd {R_j^{(outer)}}^T
\end{equation}
where
\begin{align}
\dd R_i^{(outer)}&=\sum_{1\leq s,t,j\leq k}\sum_{l=k+1}^{kn}\frac{\bs{w}_j^T\dd L\bs{w}_l\bs{u}_s^{(i)}{\bs{v}_t^{(i)}}^T}{(\sigma_s^{(i)}+\sigma_t^{(i)})(\lambda_j-\lambda_l)}\times \nonumber \\
&\qquad\Big(\big((\bs{e}_i^{(n)}\otimes I_k)\bs{u}_s^{(i)}\big)^T\bs{w}_l{\bs{e}_j^{(k)}}^T\bs{v}_t^{(i)}-\nonumber\\
&\qquad\qquad\big((\bs{e}_i^{(n)}\otimes I_k)\bs{u}_t^{(i)}\big)^T\bs{w}_l{\bs{e}_j^{(k)}}^T\bs{v}_s^{(i)}\Big).
\label{eq:derivative:14}
\end{align}
Note that since $\lambda_j<\lambda_l$ for all $j\leq k<l$ hence (\ref{eq:derivative:14}) is well-defined and computable.
\end{proposition}

\begin{proof}

\end{proof}
