# Supplementary material for: Learning Transformation Synchronization
Source: arXiv:1901.09458 source file (2019-06-04)
Supplement: Supplementary file 4 [file appendix_eigenvec_stability.tex]

\section{Eigenvector Stability}
\subsection{Notation and Roadmap of this section}\label{subSec:Notation}
In this section we consider a normalized adjacency matrix 
\begin{equation}
    \begin{split}
        A^{\star} &= D^{-\frac{1}{2}} \bar{A} D^{-\frac{1}{2}} \\
        D &= \diag(d_1, d_2, \ldots, d_n)
    \end{split}
\end{equation}
which is well known to have top eigenvalue $1$.
Assume the eigen-decomposition of $A^{\star}$
\begin{equation}\label{eq:Astar:eigendecomposition}
\begin{split}
    A^{\star} &= (\vec{s} | U) \Big( \begin{array}{cc}
        1 & \\
         & \Lambda
    \end{array} \Big) (\vec{s} | U)^T \\
    &= \vec{s} \vec{s}^T + U \Lambda U^T
\end{split}
\end{equation}
where $\vec{s} = \frac{1}{\sqrt{\sum_i d_i}} D^{\frac{1}{2}} \vec{1}$ is the top-eigenvector and $U$ encodes the other eigenvectors in its columns.

Consider matrix $A$ constructed in algorithm \ref{Alg:truncated:laplacianRS}, we can explicitly write it as
\begin{equation}\label{eq:A:def}
    \begin{split}
        A &= M^T A_0 M \\
        A_0 &= (A^{\star} \otimes I_3) + E \\
        E &= (D^{-\frac{1}{2}} \otimes I_3) N (D^{-\frac{1}{2}} \otimes I_3) \\
        M &= \diag(R_1^{\star}, R_2^{\star}, \ldots, R_n^{\star})
    \end{split}
\end{equation}

Note that $A$'s eigenvector stability is similar to $A_0$, therefore we consider $A_0$ first and then extend the result to $A$.

Assume $V$'s columns encode $A_0$'s top-3 eigenvectors, and let
$\Sigma = \diag(\mu_1, \mu_2, \mu_3)$ collects the top-3 eigenvalues of $A_0$. By construction, we have
\begin{equation}\label{eq:A:eigendecomposition}
    A_0 V = V \Sigma
\end{equation}
To bound the distance between $\sqrt{\sum_k d_k} (D^{-\frac{1}{2}} \otimes I_3) V$ and $\sqrt{\sum_k d_k} (D^{-\frac{1}{2}} \otimes I_3) (\vec{s} \otimes I_3)$, we write
\begin{equation}\label{eq:V:decompostion}
    V = (\vec{s} \otimes I_3) X + (U \otimes I_3) Y
\end{equation}
and for convenience also denote
\begin{equation}\label{eq:E11:E21}
    \begin{split}
        E_{11} &= (\vec{s} \otimes I_3)^T E (\vec{s} \otimes I_3) \\
        E_{21} &= (U \otimes I_3)^T E (\vec{s} \otimes I_3) \\
        E_{22} &= (U \otimes I_3)^T E (U \otimes I_3)
    \end{split}
\end{equation}

Denote $\lambda_i$ as the $i$-th largest eigenvalue of $A^{\star}$, this means if $E = 0$, $A_0$ will have eigenvalues $\{\lambda_i\}$, each with multiplicity three.

The rest of this section is organized as follows: lemma \ref{Lemma:eigenvalue:stability} introduces results for eigenvalue stability, lemma \ref{Lemma:X} controls the distance from $X$ to $O(3)$, lemma \ref{Lemma:Expression:Y} and lemma \ref{Lemma:Bound:Y} build an upper bound of $Y$, then theorem \ref{Theorem:eigenvector:stability} follows from these results.

\subsection{Main Results}
We first introduce the main result
\begin{theorem}\label{Theorem:eigenvector:stability}
    Adopting notations from Appendix \ref{subSec:Notation}, if
$$
\|E\| + \|E_{11}\| \leq \lambda_1 - \lambda_{2}
$$
    then there exists $Q \in O(3)$ so that
    \begin{equation}
        \|\sqrt{\sum_k d_k}(D^{-\frac{1}{2}} \otimes I_3)\Bigg(V - (\vec{s} \otimes I_3)Q\Bigg)\|_{2, \infty} = O(\epsilon_1 + \frac{c \epsilon_2 (1+\epsilon_1)}{1-c \epsilon_2} )
    \end{equation}
    where 
    \begin{equation} \label{eq:Notation}
    \begin{split}
        \epsilon_1 &\coloneqq  \left(\frac{\|E\|}{\lambda_1 - \lambda_{2} - \|E_{11}\|}\right)^2 \\
        \epsilon_2 &\coloneqq  \max_i \frac{1}{d_i} \sum_{(i, j) \in \set{E}} \|N_{ij}\| \\
        c &\coloneqq  \max_{\set{E_{good}} \subseteq \set{E} \subseteq \set{E_{all}}} c(\set{E}) \\
        c(\set{E}) &\coloneqq \|P_{\epsilon}\|_{1, \infty} \\
        P_{\epsilon} &\coloneqq  (D^{-\frac{1}{2}} U [(1+\epsilon)I - \Lambda] U^T D^{\frac{1}{2}}) \otimes I_3
    \end{split}
    \end{equation}
\end{theorem}

The following lemma introduced in \cite{} considers eigenvalue stability of $A_0$.
\begin{lem}\label{Lemma:eigenvalue:stability}
\textbf{(Eigenvalue Stability) \cite{}} Adopting notations from Appendix \ref{subSec:Notation}, if
$$
\|E\| + \|E_{11}\| \leq \lambda_1 - \lambda_{2}
$$, then for $1 \leq i \leq 3$, we have
\begin{equation}
    -\| E_{11} \| \leq \mu_i - \lambda_1 \leq \|E_{11} \| 
    + \frac{\| E \|^2 - \|E_{11} \|^2}{\lambda_1 - \lambda_{2}} 
\end{equation}
\end{lem}
The next lemma controls the distance from $X$ to $O(3)$.

\begin{lem}\label{Lemma:X}
\textbf{(Controlling $X$.)} Adopting notations from Appendix \ref{subSec:Notation}, 
if
$$
\|E\| + \|E_{11}\| \leq \lambda_1 - \lambda_{2}.
$$
then there exists $Q \in O(3)$ such that 
$$
    \|X - Q\| \leq 1 - \sqrt{1 - \left(\frac{\|E\|}{\lambda_1 - \lambda_{2} - \|E_{11}\|}\right)^2}
$$
in particular, 
$$
    \|X - Q\| \leq \left(\frac{\|E\|}{\lambda_1 - \lambda_{2} - \|E_{11}\|}\right)^2
$$
\end{lem}

\begin{lem}\label{Lemma:Expression:Y}
(\textbf{Expressing $Y$.}) Adopting notations from Appendix \ref{subSec:Notation} and \eqref{eq:Notation}, 
if
$$
\|E\| + \|E_{11}\| \leq \lambda_1 - \lambda_{2}
$$
Then for $1 \leq j \leq 3$, 
\begin{equation}
\begin{split}
    (U \otimes I_3) Y \vec{e}_j &= 
        \diag(\bs{s})\sum_{i=0}^{+\infty} \big(P_{\mu_j-1} D^{-1} N\big)^{i+1} (\vec{1} \otimes I_3) X \vec{e}_j
\end{split}
\label{Eq:Lambda:Expression}
\end{equation}
\end{lem}

\begin{lem}\label{Lemma:Bound:Y}
Adopting notations from Appendix \ref{subSec:Notation} and \eqref{eq:Notation}, if
$$
\|E\| + \|E_{11}\| \leq \lambda_1 - \lambda_{2}
$$
then 
\begin{equation}
\|\sqrt{\sum_k d_k}((D^{-\frac{1}{2}}U) \otimes I_3)Y\|_{2,\infty} = O(\frac{c \epsilon_2 (1 + \epsilon_1)}{1 - c \epsilon_2})
\label{Eq:Y:L:infty}
\end{equation}
\end{lem}

These four lemma is enough to prove Theorem \ref{Theorem:eigenvector:stability}.

The next lemma is to understand the term $\epsilon_1 + \frac{(1 + \epsilon_1) c \epsilon_2}{1 - c \epsilon_2}$.
\begin{lem}\label{lem:orders}
    Adopting notations from Appendix \ref{subSec:Notation} and \eqref{eq:Notation}, 
    assuming there exist constants $\rho > 0, c_2 > 0$, s.t. for all edge set $\set{E}$ with $\set{E}_{good} \subseteq \set{E} \subseteq \set{E}_{all}$
    $$
    1 - \lambda_2 - \epsilon_2 \geq \rho, \quad 1 - c \epsilon_2 \geq c_2
    $$
    we have
    \begin{align*}
        \epsilon_2 \leq 2, \quad \epsilon_1 \leq \frac{\epsilon_2^2}{\rho^2}
    \end{align*}
    and
    \begin{align*}
        \epsilon_1 + \frac{(1 + \epsilon_1) c \epsilon_2}{1 - c \epsilon_2} &\leq \frac{\epsilon_2^2}{\rho^2} + \frac{(1+\frac{\epsilon_2^2}{\rho^2}) c \epsilon_2}{c_2} \\
        &\leq (\frac{2}{\rho^2} + \frac{c(1+\frac{4}{\rho^2})}{c_2}) \epsilon_2
    \end{align*}
\end{lem}
The proof of this lemma is omitted.

We then begins to bound $\|R_i^t - Q^TR_i^{\star}\|$ for each iteration $t$ in the algorithm.
\begin{lem}\label{Lemma:delta} Adopting notations from Appendix \ref{subSec:Notation} and \eqref{eq:Notation}. Consider algorithm \ref{Alg:truncated:laplacianRS}, we first define
\begin{itemize}
    \item Let $\set{E}^{(t)}$ be the edge set before the $t$-th iteration, e.g. $\set{E}^{(0)} = \set{E}_{all}$, and $R_i^{(t)}$ be the value of $R_i$ after $t$-th iteration.
    \item Let 
    $$
    \epsilon_2^{(t)} \coloneqq \max_i \frac{1}{d_i} \sum_{(i, j) \in \set{E}^{(t)}} \|N_{ij}\|
    $$
    ,
    $$
        \delta^{(t)} \coloneqq \min_{Q \in O(3)}\max_i \|R_i^{(t)} - Q^T R_i^{\star}\|
    $$
    ,
    $$
        C^{(t)} \coloneqq \max_{(i, j) \in \set{E}^{(t)}} \|N_{ij}\|
    $$
    ,
    $$
        c_3 \coloneqq (\frac{2}{\rho^2} + \frac{3 c(1+\frac{4}{\rho^2})}{c_2}) + 2 (\frac{2}{\rho^2} + \frac{3 c(1+\frac{4}{\rho^2})}{c_2})^2
    $$,
    $$
        r \coloneqq \frac{d_{bad}}{d_{good}}
    $$
\end{itemize}, then the following holds
\begin{itemize}
    \item For the first iteration,
    \begin{align}
        C^{(0)} &\leq C \\
        \epsilon_2^{(0)} &\leq \sigma + C \\
        \delta^{(0)} &\leq c_3(\sigma + C) \\
        C^{(1)} &\leq \epsilon_0 + c_3 \sigma + r c_3 C
    \end{align}
    \item For $t \geq 1$, if 
    $$
    C^{(t)} \leq (\sum_{i=0}^{t-1} (rc_3)^i \tilde{c}^{t-i-1}) \epsilon_0 + c_3(\frac{1-(rc_3)^t}{1-rc_3}) \sigma + (rc_3)^t C
    $$, then
    \begin{align}
        \epsilon_2^{(t)} &\leq \sigma + r C^{(t)} \\
        & = r(\sum_{i=0}^{t-1} (rc_3)^i \tilde{c}^{t-i-1}) \epsilon_0  \\
        &+ (r c_3(\frac{1-(rc_3)^t}{1-rc_3}) + 1) \sigma + r (rc_3)^t C \\
        \delta^{(t)} &\leq c_3 \epsilon_2^{(t)} \\
        C^{(t+1)} &\leq \epsilon_0 \tilde{c}^{t-1} + \delta^{(t)} \\
        & \leq \epsilon_0 \tilde{c}^{t-1} + c_3 \epsilon_2^{(t)} \\
        &\leq [(\sum_{i=0}^{t-1} (rc_3)^{i+1} \tilde{c}^{t-i-1}) + \tilde{c}^{t-1}] \epsilon_0  \\
        &+ c_3(r c_3(\frac{1-(rc_3)^t}{1-rc_3}) + 1) \sigma + (rc_3)^{t+1} C \\
        &\leq [(\sum_{i=1}^{t} (rc_3)^{i} \tilde{c}^{t-i}) + \tilde{c}^{t-1}] \epsilon_0  \\
        &+ c_3\frac{1-(rc_3)^{t+1}}{1-rc_3} \sigma + (rc_3)^{t+1} C \\
        &\leq (\sum_{i=0}^{t} (rc_3)^{i} \tilde{c}^{t-i}) \epsilon_0  \\
        &+ c_3\frac{1-(rc_3)^{t+1}}{1-rc_3} \sigma + (rc_3)^{t+1} C
    \end{align}    
\end{itemize}
    % Let the maximum degree be $d_{\max}$, the minimal number of correct edges for each node be $d_{\textup{good}}$.
    % Define $\delta(\set{E})$ w.r.t. the current edge set $\set{E}$ as
    % $$
    %     \delta(\set{E}) \coloneqq \min_{Q \in O(3)} \max_{i} \|R_i - Q^T R_i^{\star}\|
    % $$
    % we have
    % \begin{equation}
    %     \delta(\set{E}) = O(\epsilon_1 + \frac{c \epsilon_2}{1-c \epsilon_2} (1+\epsilon_1))
    % \end{equation}

\end{lem}

\subsection{Proof of Key Lemmas}
\subsubsection{Proof of Lemma \ref{Lemma:Expression:Y}}

\begin{proof}
    From \eqref{eq:A:eigendecomposition} we have
    $$
        A_0 V = V \Sigma,
    $$
    apply \eqref{eq:V:decompostion}, we have
    $$
        A_0 ((\vec{s} \otimes I_3) X + (U \otimes I_3) Y) = ((\vec{s} \otimes I_3) X + (U \otimes I_3) Y) \Sigma
    $$
    multiply $(U \otimes I_3)^T$ from the left and apply \eqref{eq:A:def}, we have
    \begin{align}
        (U \otimes I_3)^T (A^{\star} \otimes I_3 + E) ( (\vec{s} \otimes I_3) X + (U \otimes I_3) Y) = Y \Sigma
    \end{align}
    applying \eqref{eq:E11:E21} leads to
    \begin{align}
        (\Lambda \otimes I_3) Y + E_{21} X + E_{22} Y  = Y \Sigma
    \end{align}
    for $j = 1, \ldots, 3$, multiply $\vec{e}_j$ from the right, we have
    \begin{align}
        ((\mu_j I - \Lambda \otimes I_3) - E_{22})) Y \vec{e}_j = E_{21} X \vec{e}_j
    \end{align} 
    from Lemma \ref{Lemma:eigenvalue:stability}, we have
    \begin{align}
        \|E_{22}\| &\leq \|E\| \\
        & \leq \lambda_1 - \lambda_2 - \|E_{11}\| \\
        & \leq \mu_j - \lambda_2 \\
        & \leq \|\mu_j I - (\Lambda \otimes I_3)\|
    \end{align}
    which guarantees the validity of the following Taylor expansion
    \begin{align}
        Y \vec{e}_j &= ((\mu_j I - \Lambda \otimes I_3) - E_{22}))^{-1}E_{21} X \vec{e}_j \\
        &= ((\mu_j I - \Lambda \otimes I_3)(I - (\mu_j I - \Lambda \otimes I_3)^{-1} E_{22}))^{-1} E_{21} X \vec{e}_j \\
        &= (I - (\mu_j I - \Lambda \otimes I_3)^{-1} E_{22})^{-1} (\mu_j I - \Lambda \otimes I_3)^{-1} E_{21} X \vec{e}_j \\
        &= \sum_{i=0}^{+\infty} ((\mu_j I - \Lambda \otimes I_3)^{-1} E_{22})^i (\mu_j I - \Lambda \otimes I_3)^{-1} E_{21} X \vec{e}_j
    \end{align}
    Multiply $(U \otimes I_3)$ from the left on both side and let $P_{\epsilon} =  (D^{-\frac{1}{2}} U [(1+\epsilon)I - \Lambda] U^T D^{\frac{1}{2}}) \otimes I_3$, we have
    \begin{align}
        &~~~~~(U \otimes I_3) Y \vec{e}_j \nonumber \\
        &= \sum_{i=0}^{+\infty} D^{\frac{1}{2}} (P_{\mu_j-1} D^{-1} N)^{i+1} D^{-\frac{1}{2}} (\vec{s} \otimes I_3) X \vec{e}_j \nonumber \\
        &= \frac{1}{\sqrt{\sum_k d_k}} \sum_{i=0}^{+\infty} D^{\frac{1}{2}} (P_{\mu_j-1} D^{-1} N)^{i+1} (\vec{1} \otimes I_3) X \vec{e}_j\nonumber \\
        &= \diag(\bs{s})\sum_{i=0}^{+\infty} \big(P_{\mu_j-1} D^{-1} N\big)^{i+1} (\vec{1} \otimes I_3) X \vec{e}_j
    \end{align}
\end{proof}

\subsubsection{Proof of Lemma \ref{Lemma:Bound:Y}}
\begin{proof}
From Lemma \ref{Lemma:Expression:Y}, 
    \begin{align*}
        &~~\|\sqrt{\sum_k d_k} ((D^{-\frac{1}{2}}U) \otimes I_3) Y \vec{e}_j \|_{\infty} \\
        &\leq \sum_{i=0}^{+\infty} \|\diag(\bs{1}) \big(P_{\mu_j-1} D^{-1} N\big)^{i+1} (\vec{1} \otimes I_3) X \vec{e}_j\|_{\infty} \\
        &\leq \sum_{i=0}^{+\infty} \|\diag(\bs{1})\|_{1, \infty} \|\big(P_{\mu_j-1} D^{-1} N\big)^{i+1}\|_{1, \infty} \|X\| \\
        &\leq \sum_{i=0}^{+\infty}  \|\big(P_{\mu_j-1} D^{-1} N\big)\|_{1, \infty}^{i+1} \|X\| \\
        &= \frac{\|P_{\mu_j-1} D^{-1} N\|_{1, \infty} \|X\| }{1-\|P_{\mu_j-1} D^{-1} N\|_{1, \infty}}\\
        &\leq \frac{\|P_{\mu_j-1} \|_{1, \infty} \|D^{-1} N \|_{1, \infty} \|X\| }{1-\|P_{\mu_j-1} \|_{1, \infty} \|D^{-1} N\|_{1, \infty}} \\
        &\leq \frac{\|P_{\mu_j-1} \|_{1, \infty} \max_i \frac{\sqrt{3}}{d_i} \sum_{j \in \partial{i}} \|N_{ij}\| \|X\| }{1-\|P_{\mu_j-1} \|_{1, \infty} \max_i \frac{\sqrt{3}}{d_i} \sum_{j \in \partial{i}} \|N_{ij}\|} 
    \end{align*}
Let 
\begin{align*}
    c(\set{E}) &\coloneqq \sqrt{3} \max_{\epsilon \in \set{D}}\|P_{\epsilon}\|_{1, \infty} \\
    \set{D} &\coloneqq \big[-\|E_{11}\|,~  \|E_{11}\| + \frac{\|E\|^2 - \|E_{11}\|^2}{1 - \lambda_2}\big] \\
    c &\coloneqq \max_{\set{E}_{good} \subseteq \set{E} \subseteq \set{E}_{all}}c(\set{E}) \\
    \epsilon_2 &\coloneqq \max_i \frac{1}{d_i} \sum_{j \in \partial{i}} \|N_{ij}\|
\end{align*}
and recall lemma \ref{Lemma:X}, we get
    \begin{align*}
        \|\sqrt{\sum_k d_k} ((D^{-\frac{1}{2}}U) \otimes I_3) Y \vec{e}_j \|_{\infty} &\leq \frac{c \epsilon_2 (1+\epsilon_1) }{1- c \epsilon_2 }
    \end{align*}
Combine the results for $1 \leq j \leq 3$, we have
\begin{align*}
    \|\sqrt{\sum_k d_k} ((D^{-\frac{1}{2}}U) \otimes I_3) Y \|_{2, \infty} &\leq \frac{\sqrt{3} c \epsilon_2 (1+\epsilon_1) }{1-c \epsilon_2 }
\end{align*}
\end{proof}

\subsubsection{Proof of Theorem \ref{Theorem:eigenvector:stability}}
\begin{proof}

Note that
\begin{align*}
    \|X - Q\| &\leq \frac{\|E\|^2}{(1 - \lambda_2 - \|E_{11}\|)^2} \nonumber \\
    & \leq \frac{\|D^{\frac{1}{2}}\|^2 \|(D^{-1}\otimes I_3) N\|^2 \|D^{-\frac{1}{2}}\|^2}{(1 - \lambda_2 - \|E_{11}\|)^2} \nonumber \\
    & \leq \frac{d_{\max} \epsilon_2^2}{d_{\min}(1 - \lambda_2 - \epsilon_2)^2} \nonumber \\
    & \leq \frac{d_{\max} \epsilon_2^2}{d_{\min}(\rho - \epsilon_2)^2}
\end{align*}
where 
$$
    \rho \coloneqq \min_{\set{E}_{good} \subseteq \set{E} \subseteq \set{E}_{all}} 1 - \lambda_2(\set{E})
$$
From \eqref{eq:V:decompostion} and lemma \ref{Lemma:X}, we have
\begin{align*}
    &~~~~~\|\sqrt{\sum_k d_k} (D^{-\frac{1}{2}} \otimes I_3) \Big[ V - (\vec{s} \otimes I_3)Q \Big] \|_{2, \infty}  \\
    &= \|(\vec{1} \otimes I_3)(X-Q) + \sqrt{\sum_k d_k} ((D^{-\frac{1}{2}}U) \otimes I_3)Y\|_{2, \infty} 
    \\
    & \leq \|(\vec{1} \otimes I_3)\|_{2, \infty} \|(X-Q)\| + \frac{c \epsilon_2 (1+\epsilon_1) }{1-c \epsilon_2 } \\
    & \leq  \epsilon_1 + \frac{\sqrt{3} c \epsilon_2 (1+\epsilon_1) }{1-c \epsilon_2 }
\end{align*}
\end{proof}
