# Supplementary material for: Learning Transformation Synchronization
Source: arXiv:1901.09458 source file (2019-06-04)
Supplement: Supplementary file 5 [file appendix_exact.tex]

\section{Proof of Proposition 1} \label{Appendix:A}

% Algorithm \ref{Alg:laplacianRS} constructs a block matrix $L \in \mathbb{R}^{3n \times 3n}$
% % = \Bigg(
% % \begin{array}{ccccccc}
% %     d_1 I &  & \ldots & & && \\
% %      & \ddots & & & && \\
% %     \vdots & & d_i I & \ldots & -R_{ij}^T &&\\
% %     & & \vdots & \ddots & \vdots &&\\
% %     & & -R_{ij} & \ldots & d_j I &&\\
% %     & & &  & &\ddots &  \\
% %     & & & & &&d_n I
% % \end{array} \Bigg)$, i.e. a block matrix 
% with $n \times n$ blocks, the block on $i-$th row and $j-$th column is defined as 
% \begin{equation}
%     L_{ij} = \begin{cases}
%         -R_{ij} & \textup{if }(i,j) \in E\\
%         d_i I & \textup{if } i = j \\
%         0 & \textup{otherwise}
%     \end{cases}
% \end{equation}
Recall step 2 in algorithm \ref{Alg:truncated:laplacianRS} where a block matrix $A$ is constructed. In this section, we consider the noise free setting, i.e. there exists $R_1^{\star}, R_2^{\star}, \ldots R_n^{\star} \in SO(3)$, such that $R_{ij} = (R_j^{\star})^T R_i^{\star}$. We denote the block matrix constructed from perfect correspondence $R_{ij}$ as $A^{\star}$. We can write $A^{\star}$ as
\begin{equation}
    \begin{split}
        A^{\star} & \coloneqq M^T D^{-\frac{1}{2}}\tilde{A} D^{-\frac{1}{2}} M\\
        M & \coloneqq \diag(R_1^{\star}, R_2^{\star}, \ldots,  R_n^{\star}), \quad R_i^{\star} \in SO(3) \\
        D & \coloneqq \diag(d_1I, d_2I, \ldots, d_nI) \\
        \tilde{A}_{ij} & \coloneqq \begin{cases}
            I & \textup{if }(i,j) \in \set{E}\\
            0 & \textup{otherwise}
        \end{cases}
    \end{split}
    \label{eq:A0:def}
\end{equation}
The following lemma describes $A^{\star}$'s top eigenspace.
\begin{lem}
Consider $A^{\star}$ defined in \eqref{eq:A0:def}, the following holds: 
\begin{itemize}
    \item [1)] $A^{\star}$'s eigenvalues lie in $[-1, 1]$.
    \item [2)] $A^{\star}$'s eigenspace of eigenvalue 1 is 3 dimensional and can be spanned by the columns of 
    $$
        M^T D^{\frac{1}{2}} \begin{pmatrix}
        I \\
        I \\
        \vdots \\
        I
    \end{pmatrix}
    $$
\end{itemize}

\begin{proof}
1) The statement is true since $D^{-\frac{1}{2}}\tilde{A}D^{-\frac{1}{2}}$ is a normalized adjacency matrix and $M$ is orthogonal. 

2) Since $D^{-\frac{1}{2}}\tilde{A}D^{-\frac{1}{2}}$ is a normalized adjacency matrix with 3 connected components, one can show that its eigenspace of the largest eigenvalue (i.e. 1) is exactly 3 dimensional. Since 
$$
A^{\star} M^T D^{\frac{1}{2}} \begin{pmatrix}
    I \\
    I \\
    \vdots \\
    I
\end{pmatrix} = M^T D^{\frac{1}{2}}  \begin{pmatrix}
    I \\
    I \\
    \vdots \\
    I
\end{pmatrix}
$$, we confirm that the eigenspace of eigenvalue 1 can be spanned by the columns of 
$M^T D^{\frac{1}{2}} \begin{pmatrix}
    I \\
    I \\
    \vdots \\
    I
\end{pmatrix}$.
\end{proof}
\label{lem:eigenspace}
\end{lem}

Based on Lemma \ref{lem:eigenspace}, we have 
$$
B^0 \coloneqq \frac{1}{\sqrt{\sum_i d_i}} M^T D^{\frac{1}{2}} \begin{pmatrix}
    I \\
    I \\
    \vdots \\
    I
\end{pmatrix} Q = \frac{1}{\sqrt{\sum_i d_i}} \begin{pmatrix}
    \sqrt{d_1}(R_1^{\star})^T \\
    \sqrt{d_2}(R_2^{\star})^T \\
    \vdots \\
    \sqrt{d_n}(R_n^{\star})^T
\end{pmatrix} Q
$$, where $Q$ is an orthogonal matrix and the coefficient $\frac{1}{\sqrt{\sum_i d_i}}$ comes from normalization.
The algorithm then projects $\frac{\sqrt{\sum_i d_i}}{\sqrt{d_i}}(B_i^0)^T$ onto $SO(3)$, resulting in $R_i = Q^T\det(Q) R_i^{\star}$, which completes the proof of the proposition.
