# Supplementary material for: Learning Transformation Synchronization
Source: arXiv:1901.09458 source file (2019-06-04)
Supplement: Supplementary file 6 [file appendix_proofs.tex]

\subsection{Proof of Key Lemmas}
\subsubsection{Proof of Lemma \ref{Lemma:Expression:Y}}

\begin{proof}
    From \eqref{eq:A:eigendecomposition} we have
    $$
        A_0 V = V \Sigma,
    $$
    apply \eqref{eq:V:decompostion}, we have
    $$
        A_0 ((\vec{s} \otimes I_3) X + (U \otimes I_3) Y) = ((\vec{s} \otimes I_3) X + (U \otimes I_3) Y) \Sigma
    $$
    multiply $(U \otimes I_3)^T$ from the left and apply \eqref{eq:A:def}, we have
    \begin{align}
        (U \otimes I_3)^T (A^{\star} \otimes I_3 + E) ( (\vec{s} \otimes I_3) X + (U \otimes I_3) Y) = Y \Sigma
    \end{align}
    applying \eqref{eq:E11:E21} leads to
    \begin{align}
        (\Lambda \otimes I_3) Y + E_{21} X + E_{22} Y  = Y \Sigma
    \end{align}
    for $j = 1, \ldots, 3$, multiply $\vec{e}_j$ from the right, we have
    \begin{align}
        ((\mu_j I - \Lambda \otimes I_3) - E_{22})) Y \vec{e}_j = E_{21} X \vec{e}_j
    \end{align} 
    from Lemma \ref{Lemma:eigenvalue:stability}, we have
    \begin{align}
        \|E_{22}\| &\leq \|E\| \\
        & \leq \lambda_1 - \lambda_2 - \|E_{11}\| \\
        & \leq \mu_j - \lambda_2 \\
        & \leq \|\mu_j I - (\Lambda \otimes I_3)\|
    \end{align}
    which guarantees the validity of the following Taylor expansion
    \begin{align}
        Y \vec{e}_j &= ((\mu_j I - \Lambda \otimes I_3) - E_{22}))^{-1}E_{21} X \vec{e}_j \\
        &= ((\mu_j I - \Lambda \otimes I_3)(I - (\mu_j I - \Lambda \otimes I_3)^{-1} E_{22}))^{-1} E_{21} X \vec{e}_j \\
        &= (I - (\mu_j I - \Lambda \otimes I_3)^{-1} E_{22})^{-1} (\mu_j I - \Lambda \otimes I_3)^{-1} E_{21} X \vec{e}_j \\
        &= \sum_{i=0}^{+\infty} ((\mu_j I - \Lambda \otimes I_3)^{-1} E_{22})^i (\mu_j I - \Lambda \otimes I_3)^{-1} E_{21} X \vec{e}_j
    \end{align}
    Multiply $(U \otimes I_3)$ from the left on both side and let $P_{\epsilon} =  (D^{-\frac{1}{2}} U [(1+\epsilon)I - \Lambda] U^T D^{\frac{1}{2}}) \otimes I_3$, we have
    \begin{align}
        &~~~~~(U \otimes I_3) Y \vec{e}_j \nonumber \\
        &= \sum_{i=0}^{+\infty} D^{\frac{1}{2}} (P_{\mu_j-1} D^{-1} N)^{i+1} D^{-\frac{1}{2}} (\vec{s} \otimes I_3) X \vec{e}_j \nonumber \\
        &= \frac{1}{\sqrt{\sum_k d_k}} \sum_{i=0}^{+\infty} D^{\frac{1}{2}} (P_{\mu_j-1} D^{-1} N)^{i+1} (\vec{1} \otimes I_3) X \vec{e}_j\nonumber \\
        &= \diag(\bs{s})\sum_{i=0}^{+\infty} \big(P_{\mu_j-1} D^{-1} N\big)^{i+1} (\vec{1} \otimes I_3) X \vec{e}_j
    \end{align}
\end{proof}

\subsubsection{Proof of Lemma \ref{Lemma:Bound:Y}}
\begin{proof}
From Lemma \ref{Lemma:Expression:Y}, 
    \begin{align*}
        &~~\|\sqrt{\sum_k d_k} ((D^{-\frac{1}{2}}U) \otimes I_3) Y \vec{e}_j \|_{\infty} \\
        &\leq \sum_{i=0}^{+\infty} \|\diag(\bs{1}) \big(P_{\mu_j-1} D^{-1} N\big)^{i+1} (\vec{1} \otimes I_3) X \vec{e}_j\|_{\infty} \\
        &\leq \sum_{i=0}^{+\infty} \|\diag(\bs{1})\|_{1, \infty} \|\big(P_{\mu_j-1} D^{-1} N\big)^{i+1}\|_{1, \infty} \|X\| \\
        &\leq \sum_{i=0}^{+\infty}  \|\big(P_{\mu_j-1} D^{-1} N\big)\|_{1, \infty}^{i+1} \|X\| \\
        &= \frac{\|P_{\mu_j-1} D^{-1} N\|_{1, \infty} \|X\| }{1-\|P_{\mu_j-1} D^{-1} N\|_{1, \infty}}\\
        &\leq \frac{\|P_{\mu_j-1} \|_{1, \infty} \|D^{-1} N \|_{1, \infty} \|X\| }{1-\|P_{\mu_j-1} \|_{1, \infty} \|D^{-1} N\|_{1, \infty}} \\
        &\leq \frac{\|P_{\mu_j-1} \|_{1, \infty} \max_i \frac{\sqrt{3}}{d_i} \sum_{j \in \partial{i}} \|N_{ij}\| \|X\| }{1-\|P_{\mu_j-1} \|_{1, \infty} \max_i \frac{\sqrt{3}}{d_i} \sum_{j \in \partial{i}} \|N_{ij}\|} 
    \end{align*}
Let 
\begin{align*}
    c(\set{E}) &\coloneqq \sqrt{3} \max_{\epsilon \in \set{D}}\|P_{\epsilon}\|_{1, \infty} \\
    \set{D} &\coloneqq \big[-\|E_{11}\|,~  \|E_{11}\| + \frac{\|E\|^2 - \|E_{11}\|^2}{1 - \lambda_2}\big] \\
    c &\coloneqq \max_{\set{E}_{good} \subseteq \set{E} \subseteq \set{E}_{all}}c(\set{E}) \\
    \epsilon_2 &\coloneqq \max_i \frac{1}{d_i} \sum_{j \in \partial{i}} \|N_{ij}\|
\end{align*}
and recall lemma \ref{Lemma:X}, we get
    \begin{align*}
        \|\sqrt{\sum_k d_k} ((D^{-\frac{1}{2}}U) \otimes I_3) Y \vec{e}_j \|_{\infty} &\leq \frac{c \epsilon_2 (1+\epsilon_1) }{1- c \epsilon_2 }
    \end{align*}
Combine the results for $1 \leq j \leq 3$, we have
\begin{align*}
    \|\sqrt{\sum_k d_k} ((D^{-\frac{1}{2}}U) \otimes I_3) Y \|_{2, \infty} &\leq \frac{\sqrt{3} c \epsilon_2 (1+\epsilon_1) }{1-c \epsilon_2 }
\end{align*}
\end{proof}

\subsubsection{Proof of Theorem \ref{Theorem:eigenvector:stability}}
\begin{proof}

Note that
\begin{align*}
    \|X - Q\| &\leq \frac{\|E\|^2}{(1 - \lambda_2 - \|E_{11}\|)^2} \nonumber \\
    & \leq \frac{\|D^{\frac{1}{2}}\|^2 \|(D^{-1}\otimes I_3) N\|^2 \|D^{-\frac{1}{2}}\|^2}{(1 - \lambda_2 - \|E_{11}\|)^2} \nonumber \\
    & \leq \frac{d_{\max} \epsilon_2^2}{d_{\min}(1 - \lambda_2 - \epsilon_2)^2} \nonumber \\
    & \leq \frac{d_{\max} \epsilon_2^2}{d_{\min}(\rho - \epsilon_2)^2}
\end{align*}
where 
$$
    \rho \coloneqq \min_{\set{E}_{good} \subseteq \set{E} \subseteq \set{E}_{all}} 1 - \lambda_2(\set{E})
$$
From \eqref{eq:V:decompostion} and lemma \ref{Lemma:X}, we have
\begin{align*}
    &~~~~~\|\sqrt{\sum_k d_k} (D^{-\frac{1}{2}} \otimes I_3) \Big[ V - (\vec{s} \otimes I_3)Q \Big] \|_{2, \infty}  \\
    &= \|(\vec{1} \otimes I_3)(X-Q) + \sqrt{\sum_k d_k} ((D^{-\frac{1}{2}}U) \otimes I_3)Y\|_{2, \infty} 
    \\
    & \leq \|(\vec{1} \otimes I_3)\|_{2, \infty} \|(X-Q)\| + \frac{c \epsilon_2 (1+\epsilon_1) }{1-c \epsilon_2 } \\
    & \leq  \epsilon_1 + \frac{\sqrt{3} c \epsilon_2 (1+\epsilon_1) }{1-c \epsilon_2 }
\end{align*}
\end{proof}
